# Supplementary material for: Active Huygens' Box: Metasurface-Enabled Arbitrary Electromagnetic Wave Generation Inside a Cavity
Source: arXiv:1810.05998 ancillary file (2018-10-14)
Supplement: Supplementary file 1 [file 1805_HuygensBox_Expt_v08_Supp_arxiv.pdf]

# Supplementary Information
# Active Huygens' Box: Metasurface-Enabled Arbitrary Electromagnetic Wave Generation Inside a Cavity

Alex M. H. Wong*

*Department of Electronic Engineering,*

*State Key Laboratory of Millimeter Waves,*

*City University of Hong Kong, Hong Kong SAR, China*

George V. Eleftheriades†

*The Edward S. Rogers Sr. Department of Electrical and*

*Computer Engineering, University of Toronto, Canada*

(Dated: October 14, 2018)

## Abstract

This documents contains supplementary text and figures for the main paper.

* alex.mh.wong@cityu.edu.hk

† gelefth@ece.utoronto.ca

## S1. THE TWIN CURRENT FILAMENT

This section explains the working mechanism of the twin current filament as introduced in the main text. The geometry of the metasurface element is introduced in the main text and depicted in Fig. 1b therein.

We form a simple active Huygens' metasurface using the twin current filament as the Huygens' source element. As depicted in Fig. 1b, this element consists of two line currents along the z-direction, equidistant from the metasurface boundary, which for the illustrative purpose of this subfigure runs along the y-direction. The line source with current $I_a$ is located just inside the Huygens' box, the one with current $I_b$ is located just outside.

The currents $I_a$ and $I_b$ running through this source can be separated into an even (or co-propgation) mode ($I_e$) — which corresponds to an effective electric current in the z-direction, and an odd (or counter-propagation) mode ($I_m$) — which corresponds to an effective magnetic current orthogonal to z and tangential to the metasurface direction. The even and odd mode currents are obtained from the filament currents through

$$\begin{aligned} I_e &= I_b + I_a \ , \\ I_m &= \frac{I_b - I_a}{2} \ , \end{aligned} \tag{S1}$$

and the corresponding electric and magnetic surface currents are

$$\begin{aligned} \mathbf{J_s} &= \frac{I_e}{s}\hat{\mathbf{z}} \ , \\ \mathbf{M_s} &= \frac{j\omega\mu_0 I_m w}{s}\left(\hat{\mathbf{n}} \times \hat{\mathbf{z}}\right) \ . \end{aligned} \tag{S2}$$

Here $\omega = 2\pi f$ is the angular frequency and $\mu_0$ is the permeability of free-space. As shown in Fig. 1c, $h$, $w$ and $s$ respectively denote the parallel-plate separation, line source separation and unit cell size. As introduced in the main text, $\hat{\mathbf{n}}$ points outward (i.e. from current filament a to b). Upon rearranging (S1) and (S2), we arrive at equation (2) in the main text.

## S2. THE MIRRORED CURRENT FILAMENT

This section explains the working mechanism of the mirrored current filament as introduced in the main text. Fig. 4a shows the mirrored current filament. One arrives at the mirrored current filament by dissecting the twin current filament with a perfect conductor surface. Applying electromagnetic image theory [1], one can understand that the perfect conductor surface serves as an anti-mirror to the single current filament. This effectively suppresses the electric surface current, doubles the magnetic surface current, and leaves unaffected the electromagnetic fields inside the Huygens' box. Hence, somewhat counter-intuitively, the remaining electric current filament $I$ actually excites the odd mode, which synthesizes the magnetic surface current. Mathematically, in this arrangement (2) simplifies to (4) (both equations are introduced in the main text).

## S3. A NOTE ON SUBWAVELENGTH FOCUSING USING SUPEROSCILLATIONS

Since the pioneering works from Abbé and Rayleigh on the resolution of imaging systems [2, 3], it has long been understood that the resolution of an electromagnetic wave is limited to about half its wavelength. In recent decades we witnessed the emergence of electromagnetic imaging systems with much higher resolution, which make use of evanescent electromagnetic waves, chemical fluorescent labels and other forms of prior information [4–10]. However, these methods are plagued by some combination of drawbacks, such as the requirement of prior sample preparation, fine-step scanning with step sizes of $\lambda/10$ or less, short working distance of $\lambda/10$ or less, intensive data post-processing and restriction to a very specific class of imaged objects.

Much more recently, it has been shown that propagating waves can achieve super-resolution using a wave phenomenon called superoscillation [11, 12]. By interfering slow-varying waves, regions of sharp variations can be obtained wherein the waveform oscillates faster than the fastest constituent waveform. Using this technique, researchers have demonstrated the formation of subwavelength hotspots as well as far-field super-resolution microscopes [13–20]. However, a major drawback to such superoscillation waveforms is the existence of a non-superoscillatory high-energy region [21]. The existence of this high-energy region is proven to be mathematically inevitable; further, the waveform energy is proven to scale aggressively with the rate and duration of the superoscillation feature. Example of superoscillation waveforms, constructable with propagating waves, are shown in Figs. 6a-b. The high-energy region poses a stringent limit to the rate and duration of the superoscillation. Moreover, its existence highly increases the energy and/or sensitivity cost of the super-resolution system, and can lead to spurious scattering by particles that fall in the high-energy region. While methods have been proposed to sidestep disadvantages associated with the high-energy region, its existence remains a hurdle for the widespread deployment of superoscillation-based imaging systems [22]. This work presents, to the best of our knowledge, a first work on synthesizing a subwavelength focal spot using superoscillations, without generating the accompanying high-energy region.

## S4. TOWARDS A 3D HUYGENS' BOX OF ARBITRARY SIZE AND SHAPE

In this section we offer discussion in generalizing the work towards a 3D closed surface of arbitrary size and shape. To synthesize a Huygens' box in 3D space, one needs a metasurface which can generate electric and magnetic currents in arbitrary directions. The currents can be synthesized by various sources: whereas in this work we build our active Huygens' metasurface element from ground-backed monopoles, various Huygens' sources and magnetodielectric antennas [23, 24] would also serve well as active Huygens' metasurface elements. As long as these metasurface elements are spaced less than half-wavelength apart, the metasurface satisfies the Nyquist criterion [25] and hence can faithfully synthesize all propagating waveforms. Fig. S1 demonstrates this: in this example, a plane wave is generated within a 4 × 4 wavelength Huygens' box, excited by elements which are spaced 0.4-wavelengths apart. Evidently, at this spacing, the plane wavefront is very well synthesized away from the evanescent near-field of the individual antennas. This example also shows the Huygens' box in operation over a larger area than is experimentally demonstrated in this paper.

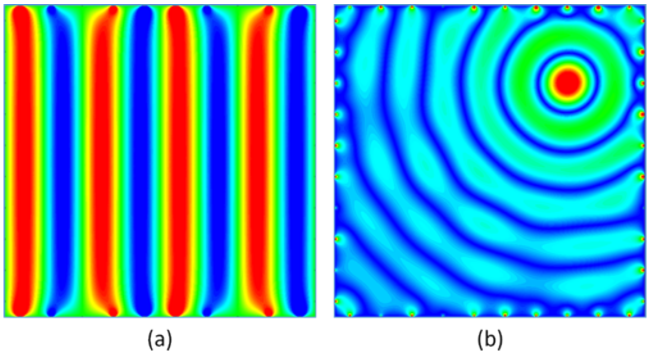


Supplementary Figure S1. Waveform generation with a large Huygens' box. Simulation results showing the generation of (a) a travelling wave with $\theta = 0$ ($E_z$ plotted at an instant in time) and (b) a Bessel wave centered at $x = \lambda$, $y = \lambda$ (phasor amplitude of $E_z$ plotted). Both waves are generated in a $4\lambda \times 4\lambda$ Huygens' box, with 10 elements on each side spaced $0.4\lambda$ apart.

## S5. BANDWIDTH ANALYSIS

We hereby briefly study the typical bandwidth for the Huygens' box. The bandwidth for an arbitrary waveform synthesis device depends on many factors, including the nature of the waveform one wishes to generate, the spectral response of the source, the tuning circuit and the metasurface element. In this work, while we design the metasurface current weights to synthesize waveforms at an operational frequency of 1 GHz, we find that waveform synthesis is achieved over a reasonable bandwidth of about 11% surrounding this frequency, both for the travelling plane wave and for the subwavelength-focused superoscillatory wave. Figs. S2 shows the experimentally measured electric field profile for the generation of four waveforms — the 45° travelling plane wave, the standing wave, the Bessel wave and the superoscillatory subwavelength focus — at frequencies of 0.92 GHz (Figs. S2a-d) and 0.96 GHz (Figs. S2e-h) 1.03 GHz (Figs. S2i-l) respectively. Despite slight deviations, the travelling plane wave is reasonably synthesized. For the superoscillatory subwavelength focus, Fig. S2m shows the focal field pattern at the image plane as a function of frequency. As shown, for a bandwidth of 11% around 1 GHz, subwavelength focusing is achieved with the selective excitation of propagating waves. While the bandwidths quoted here are achieved without spectral considerations at the design stage, the operational bandwidth of the Huygens' box can be dramatically extended when one takes care to employ broadband components and frequency-tuned excitations [24]. In this latter case, one can further tune a broadband version of the Huygens' box to achieve frequency-dependent waveforms, hence unlocking an extra dimension of waveform control of great importance to many applications.

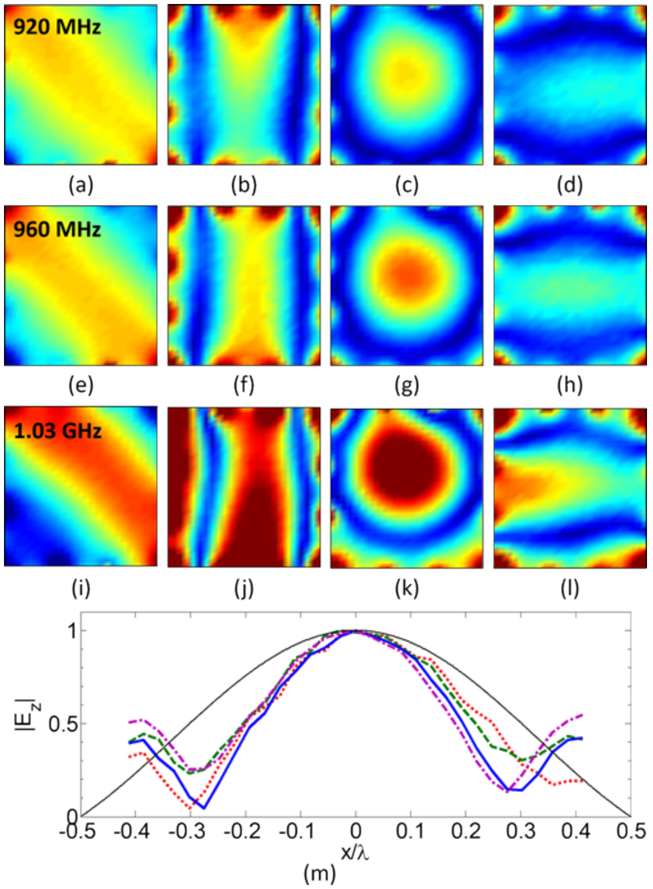


Supplementary Figure S2. Bandwidth estimation for the Huygens' box. (a-d) Experimentally measured waveform at (a-d) 920 MHz, (e-h) 960 MHz and (i-l) 1.03 GHz. The waveforms generated are a travelling wave with $\theta = 45°$ (a, e and i), a standing wave in the x- (horizontal) direction (b, f and j), (c) a Bessel waveform (c, g and k) and a superoscillation subwavelength focus (d, h and l). (m) The focal width of the superoscillation waveform as a function of frequency. The shown frequencies are 920 MHz (red, dotted), 960 MHz (green, dotted), 1 GHz (blue, solid), 1.03 GHz (purple, dashdot), and the 1 GHz diffraction limited sinc function (black, thin line).

---

[1] R. F. Harrington, *Time-Harmonic Electromagnetic Fields*, IEEE Pass Series on Electromagnetic Wave Theory (IEEE Press, 2001).

[2] E. Abbé, "Beitrge zur theorie des mikroskops und der mikroskopischen wahrnehmung." Archiv. f. mickroskopische anat. **9**, 413–168 (1873).

[3] Lord Rayleigh, "On pin-hole photography," The London, Edinburgh, and Dublin Philos. Mag. and Journal of Science **31**, 87–99 (1891).

[4] E. H. Synge, "A suggested method for extending microscopic resolution into the ultra-microscopic region," Philos. Mag. **6**, 356–362 (1928).

[5] E. A. Ash and G. Nicholls, "Super-resolution aperture scanning microscope," Nature **237**, 510–512 (1972).

[6] D. W. Pohl, W. Denk, and M. Lanz, "Optical stethoscopy: Image recording with resolution $\lambda/20$," Appl. Phys. Lett. **44**, 651–653 (1984).

[7] J. B. Pendry, "Negative refraction makes a perfect lens," Phys. Rev. Lett. **85**, 3966–3969 (2000).

[8] S. W. Hell and J. Wichmann, "Breaking the diffraction resolution limit by stimulated emission: stimulated-emission-depletion fluorescence microscopy," Opt. Lett. **19**, 780–782 (1994).

[9] M. J. Rust, M. Bates, and X. Zhuang, "Sub-diffraction-limit imaging by stochastic optical reconstruction microscopy (storm)," Nat. Methods **3**, 793–795 (2006).

[10] A. Szameit, Y. Shechtman, E. Osherovich, E. Bullkich, P. Sidorenko, H. Dana, S. Steiner, E. B. Kley, S. Gazit, T. Cohen-Hyams, S. Shoham, M. Zibulevsky, I. Yavneh, Y. C. Eldar, O. Cohen, and M. Segev, "Sparsity-based single-shot subwavelength coherent diffractive imaging," Nat. Mater. **11**, 455–459 (2012).

[11] Y. Aharonov, J. Anandan, S. Popescu, and L. Vaidman, "Superpositions of time evolutions of a quantum system and a quantum time-translation machine," Phys. Rev. Lett. **64**, 2965–2968 (1990).

[12] M. V. Berry, "Faster than Fourier," (World Scientific, Singapore, 1994) pp. 55–65.

[13] F. M. Huang, Y. Chen, F. J. Garcia de Abajo, and N. I. Zheludev, "Optical super-resolution through super-oscillations," J. Opt. A: Pure Appl. Opt. **9**, S285–S288 (2007).

[14] A. M. H. Wong and G. V. Eleftheriades, "Adaptation of schelkunoff's superdirective antenna theory for the realization of superoscillatory antenna arrays," IEEE Antennas Wireless Propag. Lett. **9**, 315–318 (2010).

[15] A. M. H. Wong and G. V. Eleftheriades, "Sub-wavelength focusing at the multi-wavelength range using superoscillations: An experimental demonstration," IEEE Trans. Antennas Propag. **59**, 4766–4776 (2011).

[16] S. Kosmeier, M. Mazilu, J. Baumgartl, and K. Dholakia, "Enhanced two-point resolution using optical eigenmode optimized pupil functions," J. Opt. **13**, 105707 (2011).

[17] E. T. F. Rogers, J. Lindberg, T. Roy, S. Savo, J. E. Chad, M. R. Dennis, and N. I. Zheludev, "A super-oscillatory lens optical microscope for subwavelength imaging," Nature Materials **11**, 432–435 (2012).

[18] A. M. H. Wong and G. V. Eleftheriades, "An optical super-microscope for far-field, real-time imaging beyond the diffraction limit," Sci. Rep. **3**, 1715 (2013).

[19] D. Tang, C. Wang, Z. Zhao, Y. Wang, M. Pu, X. Li, P. Gao, and X. Luo, "Ultrabroadband superoscillatory lens composed by plasmonic metasurfaces for subdiffraction light focusing," Laser Photonics Rev. **9**, 713–719 (2015).

[20] X. H. Dong, A. M. H. Wong, M. Kim, and G. V. Eleftheriades, "Superresolution far-field imaging of complex objects using reduced superoscillating ripples," Optica **4**, 1126–1133 (2017).

[21] P. J. S. G. Ferreira and A. Kempf, "Superoscillations: Faster than the Nyquist rate," IEEE Trans. Signal Process. **54**, 3732–3740 (2006).

[22] N. I. Zheludev, "What diffraction limit?" Nature Materials **7**, 420–422 (2008).

[23] M. Chen, M. Kim, A. M. H. Wong, and G. V. Eleftheriades, "Huygens' metasurfaces from microwaves to optics: a review," Nanophotonics **7**, 1207–1231 (2018).

[24] K. M. Luk and B. Q. Wu, "The magnetoelectric dipole — A wideband antenna for base stations in mobile communications," Proc. IEEE **100**, 2297–2307 (2012).

[25] H. Nyquist, "Certain topics in telegraph transmission theory," Trans. Am. Inst. Electr. Eng. **47**, 617–644 (1928).
